# Supplementary material for: Coherent two-dimensional spectroscopy of a Fano model
Source: arXiv:1605.08572 ancillary file (2017-09-05)
Supplement: Supplementary file 1 [file prletter-SI-v4-PRB.pdf]

# 2DES lineshape of Fano systems
# Supplemental Information

Daniel Finkelstein-Shapiro,[1,*] Felipe Poulsen,[2] Tõnu Pullerits,[1,†] and Thorsten Hansen[2,1,‡]

[1]*Division of Chemical Physics, Lund University, Box 124, 221 00 Lund, Sweden*

[2]*Department of Chemistry, University of Copenhagen, DK 2100 Copenhagen, Denmark*

This document contains the derivation of the expressions for the response functions.

**Contents**

**Details of the calculation** 2

Derivation of $\mathbf{R_1}$ 3

Derivation of $\mathbf{R_2}$ 4

Derivation of $\mathbf{R_3}$ 5

Derivation of $\mathbf{R_4}$ 6

**Summary** 6

**Plots** 7

**References** 8

## DETAILS OF THE CALCULATION

The Feynmann diagrams are:

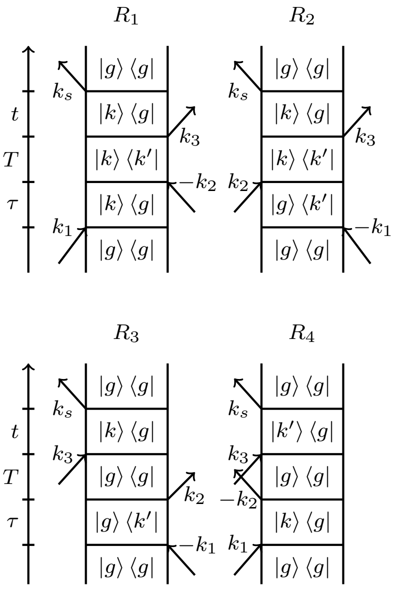


FIG. 1: Feynman pathways used to calculate the third order reponse.

$R_2$ and $R_3$ are the rephasing pathways. $R_1$ and $R_4$ are the non-rephasing pathways. The third-order polarization is written in terms of the Feynman pathways $R_i$ as:

$$P^{(3)}(t,T,\tau) = \left(\frac{i}{\hbar}\right)^3 \sum_{i=1}^{4} R_i(t,T,\tau) e^{i\omega_L t \pm i\omega_L \tau} \tag{S1}$$

In the semi impulsive limit, and assuming a Markovian bath, the third order polarization becomes proportional to the sum of the pathways. The equations for the pathways are:

$$\begin{aligned}
R_1(\tau,T,t) &= -\int dk \int dk' \mu_{gk'}\mu_{k'g}\mu_{gk}\mu_{kg} e^{-i(\omega_{kg}-i\gamma)\tau} e^{-i(\omega_{kk'}-i\eta)T} e^{-i(\omega_{kg}-i\gamma)t} \\
R_2(\tau,T,t) &= \int dk \int dk' \mu_{gk'}\mu_{k'g}\mu_{gk}\mu_{kg} e^{-i(\omega_{gk'}-i\gamma)\tau} e^{-i(\omega_{kk'}-i\eta)T} e^{-i(\omega_{kg}-i\gamma)t} \\
R_3(\tau,T,t) &= \int dk \int dk' \mu_{gk'}\mu_{k'g}\mu_{gk}\mu_{kg} e^{-i(\omega_{gk'}-i\gamma)\tau} e^{-i(\omega_{kg}-i\gamma)t} \\
R_4(\tau,T,t) &= -\int dk \int dk' \mu_{gk'}\mu_{k'g}\mu_{gk}\mu_{kg} e^{-i(\omega_{kg}-i\gamma)\tau} e^{-i(\omega_{k'g}-i\gamma)t}
\end{aligned} \tag{S2}$$

Setting the arbitrary ground state energy to zero, we write: $\omega_{kg} = \omega_k - \omega_g = \omega_k$. The transition dipole moments of excitation and relaxation are related as the complex conjugate of one another: $\mu_{gk} = \mu^*_{kg}$. Implementing the above relations, we may rewrite the set of equations for the Feynmann pathways.

$$\begin{aligned}
R_1(\tau,T,t) &= -\int dk \int dk' |\mu_{gk'}|^2 |\mu_{gk}|^2 e^{-i(\omega_k-i\gamma)\tau} e^{-i(\omega_{kk'}-i\eta)T} e^{-i(\omega_k-i\gamma)t} \\
R_2(\tau,T,t) &= \int dk \int dk' |\mu_{gk'}|^2 |\mu_{gk}|^2 e^{i(\omega_{k'}+i\gamma)\tau} e^{-i(\omega_{kk'}-i\eta)T} e^{-i(\omega_k-i\gamma)t} \\
R_3(\tau,T,t) &= \int dk \int dk' |\mu_{gk'}|^2 |\mu_{gk}|^2 e^{i(\omega_{k'}+i\gamma)\tau} e^{-i(\omega_k-i\gamma)t} \\
R_4(\tau,T,t) &= -\int dk \int dk' |\mu_{gk'}|^2 |\mu_{gk}|^2 e^{-i(\omega_k-i\gamma)\tau} e^{-i(\omega_{k'}-i\gamma)t}
\end{aligned} \tag{S3}$$

We use the Fourier transform:

$$\tilde{f}(\omega) = \int_{-\infty}^{\infty} dt f(t) e^{i\omega t}$$
$$\tilde{f}(t) = \frac{1}{2\pi} \int_{-\infty}^{\infty} d\omega \tilde{f}(\omega) e^{-i\omega t} \tag{S4}$$

Fourier transforming with respect to $t$ and $\tau$, we obtain:

$$R_1(\omega_\tau, T, \omega_t) = -\int dk \int dk' |\mu_{gk'}|^2 |\mu_{gk}|^2 \frac{e^{-i(\omega_{kk'} - i\eta)T}}{(\omega_\tau - \omega_k + i\gamma)(\omega_t - \omega_k + i\gamma)}$$
$$R_2(\omega_\tau, T, \omega_t) = \int dk \int dk' |\mu_{gk'}|^2 |\mu_{gk}|^2 \frac{e^{-i(\omega_{kk'} - i\eta)T}}{(\omega_\tau - \omega_{k'} - i\gamma)(\omega_t - \omega_k + i\gamma)}$$
$$R_3(\omega_\tau, T, \omega_t) = \int dk \int dk' |\mu_{gk'}|^2 |\mu_{gk}|^2 \frac{1}{(\omega_\tau - \omega_{k'} - i\gamma)(\omega_t - \omega_k + i\gamma)} \tag{S5}$$
$$R_4(\omega_\tau, T, \omega_t) = -\int dk \int dk' |\mu_{gk'}|^2 |\mu_{gk}|^2 \frac{1}{(\omega_\tau - \omega_k + i\gamma)(\omega_t - \omega_{k'} + i\gamma)}$$

The four equations may be solved by integrating in the complex plane. We set $|\mu_{gk}|^2 = \mu_0^2 \frac{(\epsilon_k+q)^2}{\epsilon_k^2+1}$. We assume a linear dispersion, $k = n\omega_k$, and we use $\omega_k = \epsilon_k \gamma_e + \omega_e$.

## Derivation of $\mathbf{R_1}$

$$R_1(\omega_\tau, T, \omega_t) = -(\mu_0^2 n)^2 \gamma_e^2 e^{-\eta T} I_1 I_2 \tag{S6}$$

with:

$$I_1 = \int d\epsilon_k \frac{e^{-i\epsilon_k \gamma_e T}(\epsilon_k + q)^2}{(\omega_\tau - \epsilon_k\gamma_e - \omega_e + i\gamma)(\omega_t - \epsilon_k\gamma_e - \omega_e + i\gamma)(\epsilon_k^2 + 1)}$$
$$I_2 = \int d\epsilon_{k'} \frac{e^{i\epsilon_{k'}\gamma_e T}(\epsilon_{k'} + q)^2}{(\epsilon_{k'}^2 + 1)} \tag{S7}$$

$I_1$ may be integrated using the residue theorem with a closed contour in the lower half complex plane:

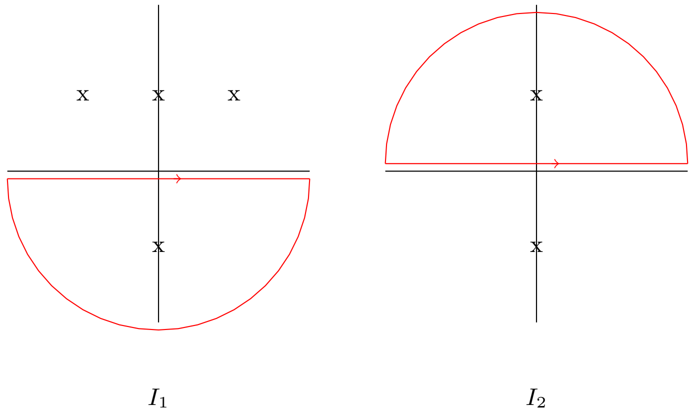


FIG. 2: The poles and the chosen contour of integration for two integrals $I_1$ and $I_2$. The contours are chosen so that the integral along the infinite semicircle vanishes.

$$I_1 = \int_{\text{arc}} - \oint = \frac{\pi(q-i)^2 e^{-\gamma_e T}}{(\omega_\tau - \omega_e + i(\gamma_e + \gamma))(\omega_t - \omega_e + i(\gamma_e + \gamma))} \tag{S8}$$

where the open contour integral along the arc vanishes. $I_2$ may be integrated using the residue theorem with a closed contour in the upper half complex plane:

$$I_2 = \oint - \int_{\text{arc}} = \pi(q+i)^2 e^{-\gamma_e T} \tag{S9}$$

where the open contour integral along the arc vanishes again.

Making the substitutions $\Gamma = \frac{\gamma_e}{\gamma_e+\gamma}$ and $\epsilon_t = \frac{\omega_t-\omega_e}{\gamma_e+\gamma}$, we finally find:

$$R_1(\epsilon_\tau, T, \epsilon_t) = (\mu_0^2 n\pi)^2 \frac{\Gamma^2(q^2+1)^2 e^{-(2\gamma_e+\eta)T}}{(\epsilon_\tau+i)(\epsilon_t+i)} \tag{S10}$$

## Derivation of $\mathbf{R_2}$

$$R_2(\omega_\tau, T, \omega_t) = (\mu_0^2 n)^2 \gamma_e^2 e^{-\eta T} I_1 I_2 \tag{S11}$$

with:

$$\begin{aligned} I_1 &= \int d\epsilon_k \frac{(\epsilon_k+q)^2 e^{-i\epsilon_k\gamma_e T}}{(\epsilon_k^2+1)(\omega_t-\epsilon_k\gamma_e-\omega_e+i\gamma)} \\ I_2 &= \int d\epsilon_{k'} \frac{(\epsilon_{k'}+q)^2 e^{i\epsilon_{k'}\gamma_e T}}{(\epsilon_{k'}^2+1)(\omega_\tau-\epsilon_{k'}\gamma_e-\omega_e-i\gamma)} \end{aligned} \tag{S12}$$

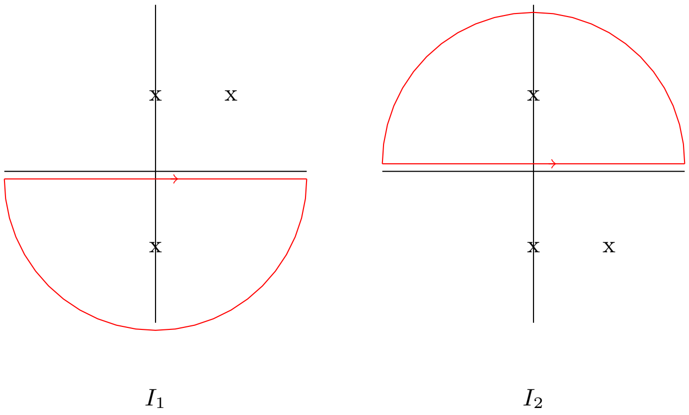


FIG. 3: The poles and the chosen contour of integration for two integrals $I_1$ and $I_2$. The contours are chosen so that the integral along the infinite semicircle vanishes.

$I_1$ may be integrated using the residue theorem with a closed contour in the lower half complex plane:

$$I_1 = \int_{\text{arc}} - \oint = \frac{\pi(q-i)^2 e^{-\gamma_e T}}{\omega_t-\omega_e+i(\gamma_e+\gamma)} \tag{S13}$$

where the open contour integral along the arc vanishes. $I_2$ may be integrated using the residue theorem with a closed contour in the upper half complex plane:

$$I_2 = \oint - \int_{\text{arc}} = \frac{\pi(q+i)^2 e^{-\gamma_e T}}{\omega_\tau-\omega_e-i(\gamma_e+\gamma)} \tag{S14}$$

where the open contour integral along the arc vanishes again.

Making the substitutions $\Gamma = \frac{\gamma_e}{\gamma_e+\gamma}$ and $\epsilon_t = \frac{\omega_t-\omega_e}{\gamma_e+\gamma}$, we finally find:

$$R_2(\epsilon_\tau, T, \epsilon_t) = (\mu_0^2 n\pi)^2 \frac{\Gamma^2(q^2+1)^2 e^{-(2\gamma_e+\eta)T}}{(\epsilon_\tau-i)(\epsilon_t+i)} \tag{S15}$$

## Derivation of $\mathbf{R_3}$

$$R_3(\omega_\tau, T, \omega_t) = (\mu_0^2 n)^2 \gamma_e^2 I_1 I_2 \tag{S16}$$

with:

$$\begin{aligned} I_1 &= \int d\epsilon_k \frac{(\epsilon_k + q)^2}{(\epsilon_k^2 + 1)(\omega_t - \epsilon_k \gamma_e - \omega_e + i\gamma)} \\ I_2 &= \int d\epsilon_{k'} \frac{(\epsilon_{k'} + q)^2}{(\epsilon_{k'}^2 + 1)(\omega_\tau - \epsilon_{k'} \gamma_e - \omega_e - i\gamma)} \end{aligned} \tag{S17}$$

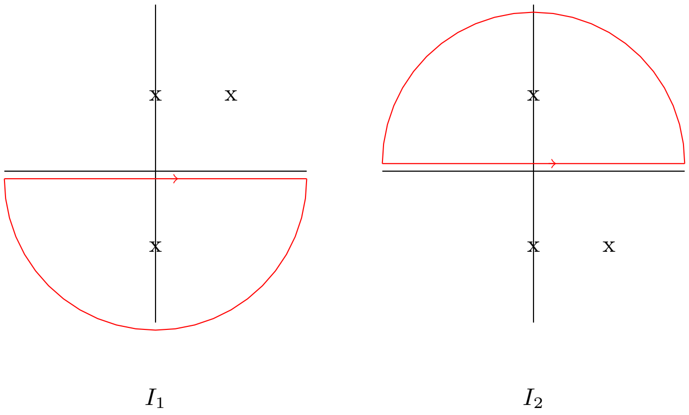


FIG. 4: The poles and the chosen contour of integration for two integrals $I_1$ and $I_2$. The contribution of the infinite semicircle is $-i\pi/\gamma_e$.

$I_1$ may be integrated using the residue theorem with a closed contour in the lower half complex plane:

$$I_1 = \int_{\text{arc}} - \oint = \frac{-i\pi}{\gamma_e} + \frac{\pi(q-i)^2}{\omega_t - \omega_e + i(\gamma_e + \gamma)} \tag{S18}$$

$I_2$ may be integrated using the residue theorem with a closed contour in the upper half complex plane:

$$I_2 = \oint - \int_{\text{arc}} = \frac{\pi(q+i)^2}{\omega_\tau - \omega_e - i(\gamma_e + \gamma)} + \frac{i\pi}{\gamma_e} \tag{S19}$$

Making the substitutions $\Gamma = \frac{\gamma_e}{\gamma_e + \gamma}$ and $\epsilon_t = \frac{\omega_t - \omega_e}{\gamma_e + \gamma}$, we finally find:

$$R_3(\epsilon_\tau, T, \epsilon_t) = (\mu_0^2 n \pi)^2 h^*(\epsilon_t) h(\epsilon_\tau) \tag{S20}$$

where $h(\epsilon)$ is the function:

$$\begin{aligned} h(\epsilon) &= \frac{\Gamma(q+i)^2 + i(\epsilon - i)}{\epsilon - i} \\ &= \Gamma \frac{\epsilon(q^2-1) - 2q}{\epsilon^2 + 1} + i\left[\frac{(q_{\text{eff}} + \epsilon)^2}{\epsilon^2 + 1} + \frac{C}{\epsilon^2 + 1}\right] \end{aligned} \tag{S21}$$

where $C = (1-\Gamma)(1+q^2\Gamma)$ and $q_{\text{eff}} = q\Gamma$. We see that the imaginary part of $h$ is the generalized Fano equation:

$$f(\epsilon, q_{\text{eff}}, C) = \frac{(q_{\text{eff}} + \epsilon)^2}{\epsilon^2 + 1} + \frac{C}{\epsilon^2 + 1} \tag{S22}$$

## Derivation of $\mathbf{R_4}$

$$R_4(\omega_\tau, T, \omega_t) = (\mu_0^2 n)^2 \gamma_e^2 I_1 I_2 \tag{S23}$$

with:

$$\begin{aligned} I_1 &= \int d\epsilon_k \frac{(\epsilon_k + q)^2}{(\epsilon_k^2 + 1)(\omega_\tau - \epsilon_k \gamma_e - \omega_e + i\gamma)} \\ I_2 &= \int d\epsilon_{k'} \frac{(\epsilon_{k'} + q)^2}{(\epsilon_{k'}^2 + 1)(\omega_t - \epsilon_{k'} \gamma_e - \omega_e + i\gamma)} \end{aligned} \tag{S24}$$

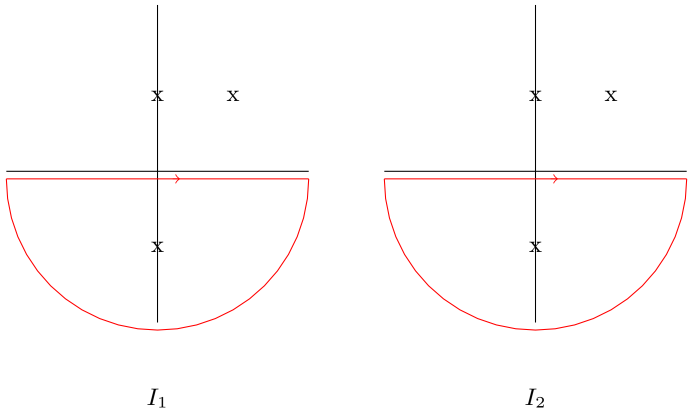


FIG. 5: The poles and the chosen contour of integration for two integrals $I_1$ and $I_2$. The contribution of the infinite semicircle is $-i\pi/\gamma_e$.

$I_1$ may be integrated using the residue theorem with a closed contour in the lower half complex plane:

$$I_1 = \int_{\text{arc}} - \oint = \frac{-i\pi}{\gamma_e} + \frac{\pi(q-i)^2}{\omega_\tau - \omega_e + i(\gamma_e + \gamma)} \tag{S25}$$

$I_2$ may be integrated using the residue theorem with a closed contour in the lower half complex plane:

$$I_2 = \int_{\text{arc}} - \oint = \frac{-i\pi}{\gamma_e} + \frac{\pi(q-i)^2}{\omega_t - \omega_e + i(\gamma_e + \gamma)} \tag{S26}$$

Making the substitutions $\Gamma = \frac{\gamma_e}{\gamma_e + \gamma}$ and $\epsilon_t = \frac{\omega_t - \omega_e}{\gamma_e + \gamma}$, we finally find:

$$R_4(\epsilon_\tau, T, \epsilon_t) = -(\mu_0^2 n\pi)^2 h^*(\epsilon_t) h^*(\epsilon_\tau) \tag{S27}$$

## SUMMARY

In summary, the four response functions are:

$$R_1(\epsilon_\tau, T, \epsilon_t) = -(\mu_0^2 n\pi)^2 \frac{\Gamma^2 (q^2+1)^2 e^{-(2\gamma_e + \eta + 1/T_{\text{pop}})T}}{(\epsilon_\tau + i)(\epsilon_t + i)} \tag{S28}$$

$$R_2(\epsilon_\tau, T, \epsilon_t) = (\mu_0^2 n\pi)^2 \frac{\Gamma^2 (q^2+1)^2 e^{-(2\gamma_e + \eta + 1/T_{\text{pop}})T}}{(\epsilon_\tau - i)(\epsilon_t + i)} \tag{S29}$$

$$R_3(\epsilon_\tau, T, \epsilon_t) = (\mu_0^2 n\pi)^2 h^*(\epsilon_t) h(\epsilon_\tau) \tag{S30}$$

$$R_4(\epsilon_\tau, T, \epsilon_t) = -(\mu_0^2 n\pi)^2 h^*(\epsilon_t) h^*(\epsilon_\tau) \tag{S31}$$

The population relaxation to the ground state, assumed to be independent of the energy of the excited state is added as an additional decay rate $1/T_{\text{pop}}$ during the evolution populaton time $T$ for those pathways that evolve along the excited state manifold during $T$.

**PLOTS**

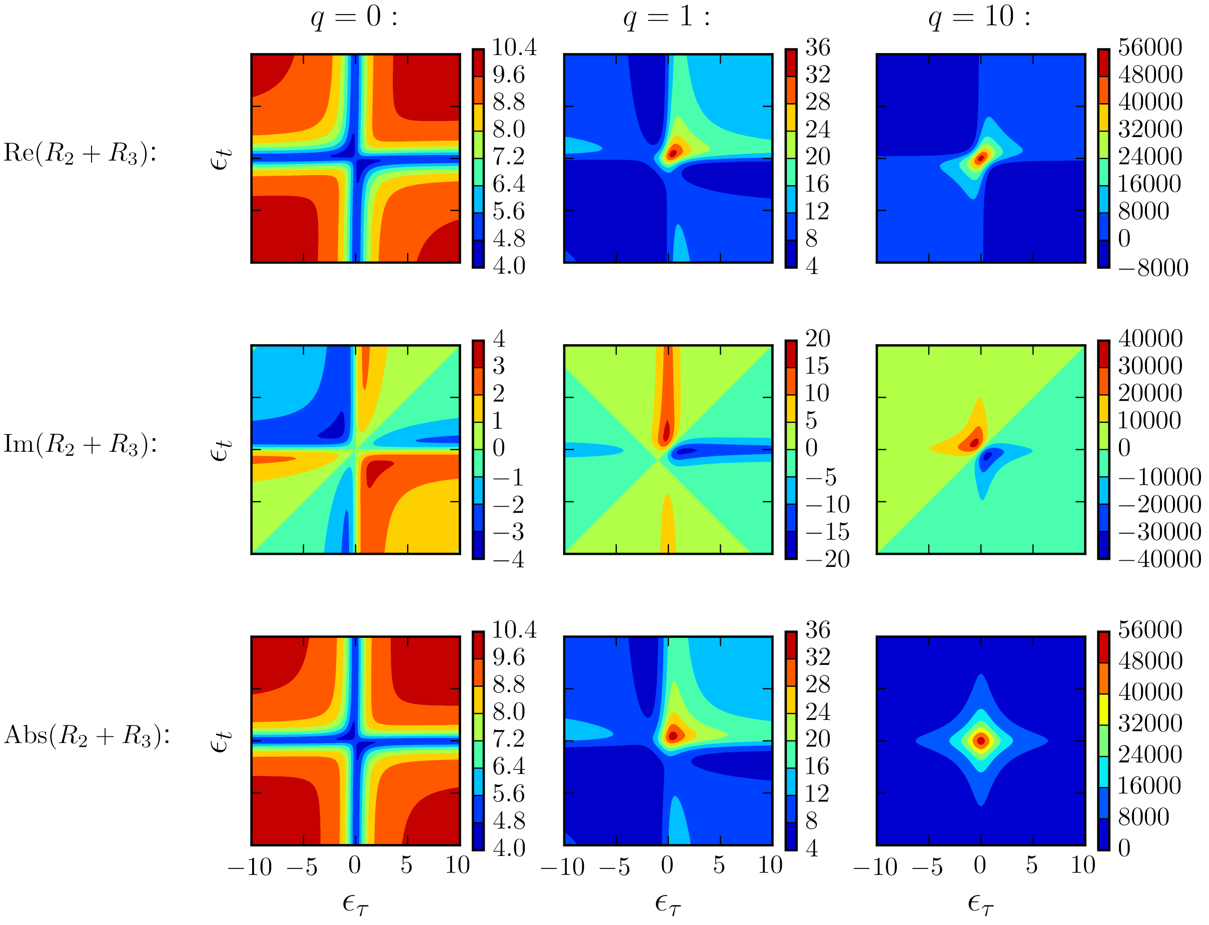


FIG. 6: Rephasing spectra for $q = 0, 1, 10$ with parameters $\gamma_e = \gamma = n = \mu_0^2 = 1$ and $T = 0$

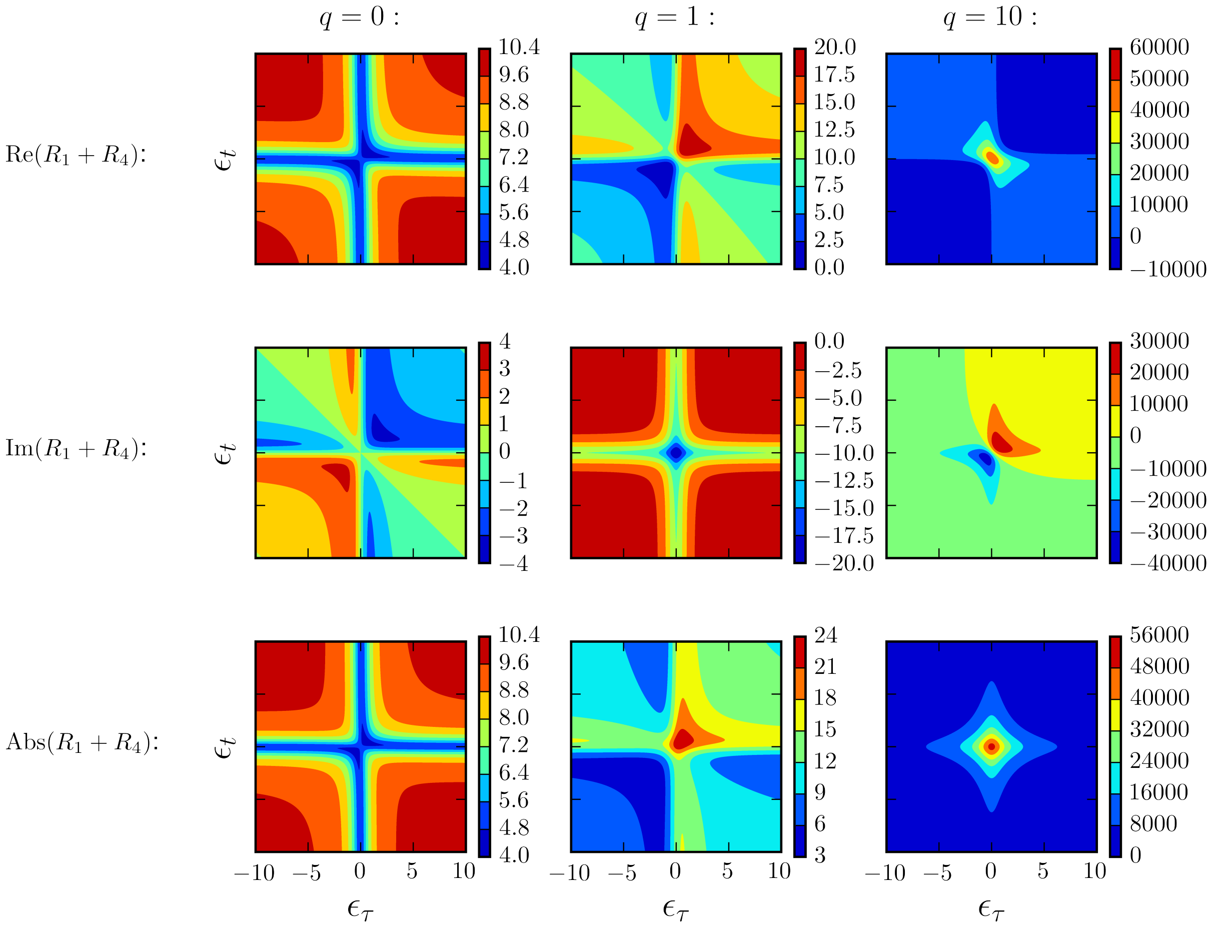


FIG. 7: Non-rephasing spectra for $q = 0, 1, 10$ with parameters $\gamma_e = \gamma = n = \mu_0^2 = 1$ and $T = 0$


* Corresponding author: daniel.finkelstein_shapiro@chemphys.lu.se
† Corresponding author: tonu.pullerits@chemphys.lu.se
‡ Corresponding author: thorsten@chem.ku.dk
